# Supplementary material for: Self-triggered strong-field QED collisions in laser-plasma interaction
Source: arXiv:2408.13238 source file (2024-08-23)
Supplement: Supplementary file 1 [file Supplemental_Material_for_Self_triggered_strong-field_QED_collisions_in_laser_plasma_interaction.pdf]

# Supplemental Material for
# "Self-triggered strong-field QED collisions in laser-plasma interaction"

Aimé Matheron,[1] Igor Andriyash,[1] Xavier Davoine,[2,3] Laurent Gremillet,[2,3] Mattys Pouyez,[4] Mickael Grech,[5] Livia Lancia,[5] Kim Ta Phuoc,[6] and Sébastien Corde[1,7,*]

[1]*LOA, ENSTA Paris, CNRS, Ecole Polytechnique, Institut Polytechnique de Paris, 91762 Palaiseau, France*
[2]*CEA, DAM, DIF, 91297 Arpajon, France*
[3]*Université Paris-Saclay, CEA, LMCE, 91680 Bruyères-le-Châtel, France*
[4]*LULI, Sorbonne Université, CNRS, CEA, Ecole Polytechnique, Institut Polytechnique de Paris, F-75255 Paris, France*
[5]*LULI, CNRS, CEA, Sorbonne Université, Ecole Polytechnique, Institut Polytechnique de Paris, F-91120 Palaiseau, France*
[6]*Univ. Bordeaux, CNRS, CEA, CELIA (Centre Lasers Intenses et Applications), UMR 5107, F-33400 Talence, France*
[7]*SLAC National Accelerator Laboratory, Menlo Park, CA 94025, USA*

(Dated: August 23, 2024)

## S1. SIMULATION CODES AND PARAMETERS

The full start-to-end simulation has been computed using three different PIC codes: FBPIC [1], HiPACE++ [2] and CALDER [3, 4], the latter one including strong-field QED processes with the SFQEDtoolkit [5]. In this section, we discuss in more details the physics of each part of the simulation, how the codes are particularly suited for each stage of the concept and detail the numerical modelling and parameters.

The simulation starts with FBPIC which models how the laser enters into the plasma together with the electron injection in the wake. FBPIC code is a full PIC code particularly suited to model laser-plasma accelerators. It uses a spectral algorithm that, in contrast to finite-difference schemes, is free from numerical dispersion in vacuum and thus models the laser propagation and its group and phase velocities more accurately, a property particularly well suited to model the physics of electron injection in laser-plasma accelerators. FBPIC performs an azimuthal decomposition where the fields are described in terms of angular modes, and in this study only the $m = 0$, $m = 1$ and $m = 2$ modes are simulated, which is sufficient to model the linear polarization of the laser and the close-to-cylindrical symmetry of the system. With only 3 modes to simulate, FBPIC is much faster than a full 3D simulation, while maintaining very good accuracy for the injection stage of our study.

The laser first propagates in vacuum from $z = 0$ to $z = 0.3\,\mathrm{mm}$ where it enters the plasma via an upramp located between $z = 0.3\,\mathrm{mm}$ and $z = 1.3\,\mathrm{mm}$. In this upramp, the plasma density rises linearly from 0 to $n_e^0 = 1 \times 10^{17}\,\mathrm{cm}^{-3}$. The plasma density is then constant at $n_e^0 = 1 \times 10^{17}\,\mathrm{cm}^{-3}$ from $z = 1.3\,\mathrm{mm}$ to $z = 2.3\,\mathrm{mm}$. Between $z = 2.3\,\mathrm{mm}$ and $2.5\,\mathrm{mm}$, the density decreases linearly from $n_e^0 = 1 \times 10^{17}\,\mathrm{cm}^{-3}$ to $n_e^0 = 7 \times 10^{16}\,\mathrm{cm}^{-3}$. The electron beam injection takes place in this $200\,\mu\mathrm{m}$ downramp, whose parameters are chosen to match typical experimental setups [6] and lead to small energy spreads for the injected beams, a key property to ensure that all electrons will experience similar $\chi_e$ values during the final QED collision. After injection in the downramp, the electron beam is then accelerated from $z = 2.5\,\mathrm{mm}$ to $z = 10\,\mathrm{mm}$ in the constant plasma density $n_e^0 = 7 \times 10^{16}\,\mathrm{cm}^{-3}$. The cylindrical FBPIC simulation domain extends over $212\,\mu\mathrm{m}$ along the longitudinal coordinate $z$, $297\,\mu\mathrm{m}$ along the radial coordinate $r$, and contains a total of $6432 \times 892$ cells in the $z$ and $r$ direction respectively. The time step is 0.11 fs. The number of macroparticles per cell is 12, uniformly distributed as $1 \times 2 \times 6$ along $z$, $r$, and $\theta$. The plasma is obtained by laser ionization of atomic hydrogen gas that is initialized in the FBPIC simulation with a parabolic transverse profile with $n_e(r) = n_e^0 \left(1 + \frac{r^2}{r_c^2}\right)$ and $r_c = 182\,\mu\mathrm{m}$.

Because of the high computational cost needed to model the electron acceleration over a long propagation distance, 40 cm for the laser-plasma accelerator in this study, a different code is used to model electron acceleration over this distance. HiPACE++ is based on the quasistatic approach, a reduced model that assumes that the driver (here the laser envelope) and the wake evolve slowly compared to the time scale of the plasma response. This quasistatic reduced model allows HiPACE++ to simulate the laser-plasma accelerator in 3D over a long distance at a much

* Corresponding authors:
aime.matheron@polytechnique.edu
sebastien.corde@polytechnique.edu

reduced computational cost. While HiPACE++ is perfectly suited to provide a highly accurate description of the physics involved in the acceleration of the electron beam, the injection process fundamentally breaks the quasistatic approximation, which explains why a different code, FBPIC, is used for the injection stage. Note that the choice of FBPIC to model the injector is also motivated by the availability of the LASY tool [7], a platform that allows to easily transfer from one PIC code to another, and used here to transfer the particles and the fields from FBPIC to HiPACE++. In HiPACE++, a laser-envelope solver is used to model the propagation of the laser pulse, accounting for the evolution of the complex field envelope and capturing the temporal phase and the spectral dynamics [8].

The HiPACE++ simulation covers the propagation distance from $z = 10\,\mathrm{mm}$ to $z = 406\,\mathrm{mm}$ and considers a pre-ionized plasma with an electron temperature of $1\,\mathrm{eV}$, a constant on-axis plasma density $n_e^0 = 7 \times 10^{16}\,\mathrm{cm}^{-3}$ and the same parabolic transverse profile for the plasma density as for the FBPIC simulation (see above), to guide the laser pulse. The 3D simulation domain extends over $200\,\mu\mathrm{m}$ longitudinally (along the comoving coordinate $\xi = z - ct$) and $500\,\mu\mathrm{m}$ transversely (along the $x$ and $y$ coordinates) for a total of $512 \times 512 \times 1280$ cells in $x$, $y$, and $\xi$ respectively. At each time step, the full plasma response is computed in the $(x, y, \xi)$ domain by integrating over $\xi$ and using 1 macroparticle per 2D $(x, y)$ cell. Cubic interpolation is used to project particles' density and current on the simulation mesh. The laser and electron beam are then advanced with a time step of $333\,\mathrm{fs}$.

The output of the HiPACE++ simulation is then transferred to CALDER which is necessary to model with high accuracy the QED processes during the collision. In this transfer, positions and momenta of individual beam electrons are accounted for as well as the laser intensity spatial and temporal envelopes, and the laser frequency chirp ($\omega$ versus $\xi$) is simplified to a linear chirp. With the CALDER 3D PIC code including SFQEDtoolkit, the full 3D physics is captured without the use of reduced models, which allows to model the laser self-focusing with high accuracy as well as the QED collision. This computationally-demanding simulation is run over a limited propagation distance of $1.5\,\mathrm{mm}$.

In the CALDER simulation, the laser enters the simulation box from the left boundary while the simulation box is fixed in the laboratory frame. The electron beam is initialized in the simulation box and is initially frozen so that the laser can pass through the electron beam. Once the laser reaches its desired location in the right part of the simulation box (the same as in the HiPACE++ simulation), we unfreeze the electron beam and the simulation switches to a moving window approach. However, to avoid any artefacts on the electron beam due to the absence of the beam self-field initialization, we enforce a ballistic propagation for the first $20\,\mu\mathrm{m}$, after which electrons evolve according their relativistic equation of motion with the electromagnetic fields of the simulation. The CALDER simulation considers a pre-ionized plasma with transversely uniform density (no parabolic channel), and starts with a $250\,\mu\mathrm{m}$ upramp where the plasma electron density linearly rises from $7 \times 10^{16}\,\mathrm{cm}^{-3}$ to $7 \times 10^{18}\,\mathrm{cm}^{-3}$. The plasma density is then constant (both transversely and along the propagation direction) and equal to $7 \times 10^{18}\,\mathrm{cm}^{-3}$ over $1.2\,\mathrm{mm}$. The plasma mirror is located at the end of this plasma density plateau.

The plasma mirror is modeled by taking advantage of the reflective condition at the right boundary of the simulation box, and by stopping the simulation window when this right boundary has reached the desired location of the plasma mirror. Once the moving window is stopped, the electron beam and laser pulse propagate towards the right boundary, and the laser is reflected by this boundary. This approach provides an idealized model for the laser reflection on the plasma mirror. Note that while the boundary conditions are set to be reflective for electromagnetic fields (except for the left boundary which is open due to the use of the moving window), they are absorbing for the particles. The collision between beam electrons and the reflected laser is modeled with high accuracy using SFQEDtoolkit. The 3D simulation box extends over $380\,\mu\mathrm{m}$ transversely (along the $x$ and $y$ coordinates) and $150\,\mu\mathrm{m}$ longitudinally (along the $z$ coordinate) and contains $380 \times 380 \times 1875$ cells in $x$, $y$ and $z$ respectively. The time step is $0.26\,\mathrm{fs}$, the electron beam is described by $2.8 \times 10^5$ macroparticles (corresponding to more than 100 macroparticles per cell in the electron beam core), and 3 macroparticles per cell are used for plasma electrons. Ions are assumed to be motionless. Collisions are not included in the simulation.

## S2. HIGH-RESOLUTION CALDER SIMULATION OF THE PLASMA MIRROR

To keep reasonable computational costs, our approach was to used a separate CALDER simulation to model a more realistic reflection of the laser on the solid-density plasma mirror and validate the main simulation. This additional simulation is performed in 3D with a much finer spatial and temporal resolution to resolve the plasma dynamics of the solid density, and only includes the laser reflection stage. It takes as an input the laser field after the self-focusing in the intensity booster: the laser is extracted from the main CALDER simulation just before the reflection and then initialized in this separate high-resolution simulation. The plasma mirror has a flat-top profile at solid density located between $z = 0$ and $z = 2\,\mu\mathrm{m}$ and an exponential ramp of the form $n_e(z) = n_c \exp(z/L_g)$ for $z < 0$ to reproduce the creation of a preplasma [9] that could degrade the reflection, with $n_c = 1.8 \times 10^{19}\,\mathrm{cm}^{-3}$ the critical density and $L_g = 56\,\mathrm{nm}$ the gradient scale length. The solid target is modeled using the $Al^{3+}$ electron density $n_e = 1.8 \times 10^{23}\,\mathrm{cm}^{-3}$,

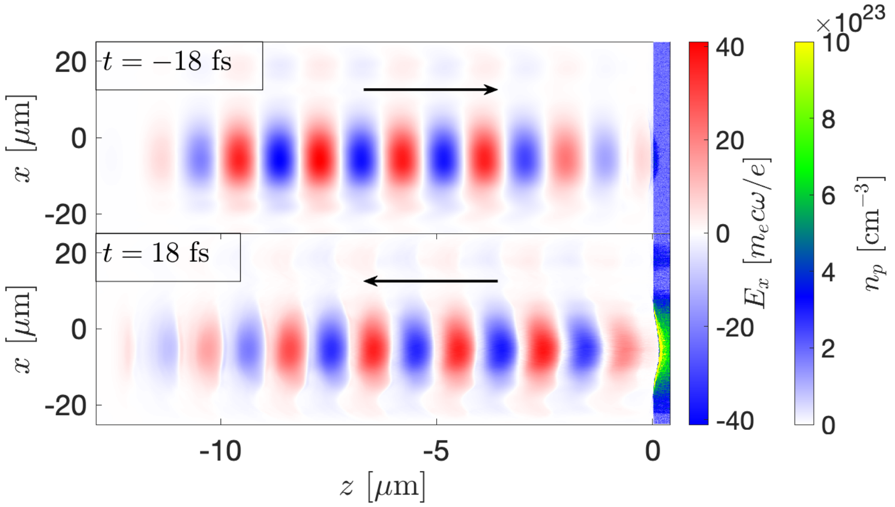


FIG. S1. Laser reflection on the plasma mirror. The 2D maps of the incident (top) and reflected (bottom) laser are shown together with the solid density plasma. Figure 3 of the main paper shows on-axis lineouts of the incident and reflected electric field in this figure.

and by enabling laser ionization of aluminum via the ADK model in the CALDER simulation [10]. The 3D simulation box extends over 50 $\mu$m transversely (along the $x$ and $y$ coordinates) and 15 $\mu$m longitudinally (along the $z$ coordinate) and contains $2660 \times 2660 \times 1591$ cells in $x$, $y$ and $z$ respectively. The simulation box is fixed. The time step is 25 as, 1 macroparticle per cell is used for plasma ions and 5 macroparticles per cell are used for plasma electrons. Collisions between electrons and between ions and electrons are modelled. Figure S1 shows 2D maps of the incident (top, at $t = -18$ fs) and reflected (bottom, at $t = 18$ fs) laser electric field. At $t = 18$ fs the laser has been fully reflected by the Al target. We see a small degradation of the sinusoidal profile of the laser electric field, due to weak harmonic generation, associated to a slight reduction of its maximum field value (by 7 % as shown in Fig. 3 of the main paper). Accounting for the reflection on the plasma mirror, $\chi_e$ is only reduced by about 7%, which justifies the approximation of perfect reflection used in the main CALDER simulation.

## S3. THEORETICAL PREDICTION OF THE NUMBER OF PRODUCED PAIRS

A simplified model has been recently proposed [11] to predict the number of pairs produced in electromagnetic showers developing in the head-on collision of an electron beam with an ultra-high intensity laser pulse under conditions relevant to forthcoming multi-petawatt laser facilities. For this study, where the electron beam transverse extension is smaller than that of the colliding laser beam (thin seed-particle beam limit), the model provides us with the shower multiplicity in a one-dimensional geometry which allows to compute the number of produced pairs per incident electron directly. We consider the simplest picture of an 11 GeV mono-energetic electron beam colliding with a laser pulse of relativistic field strength $a_0 = 40$, central wavelength $\lambda_0 = 0.8\,\mu$m and FWHM pulse duration $\tau_p = 20$ fs. The laser has a truncated $\sin^2$ temporal profile in intensity, that is nonzero only inside a 40 fs window centered on the peak laser intensity. The model predicts a multiplicity of $\sim 0.19$ [1], consistent with a produced positron charge 0.22 times that of the initial electron beam obtained in our 3D QED-PIC simulation. Accounting for the exact laser profile and initial electron beam energy distribution in the model allows for a better agreement with the 3D QED-PIC simulation, with the multiplicity reaching $(0.21 \pm 0.01)$ for the perfect reflection of the electromagnetic fields extracted from the simulation (Fig. 2 of the Manuscript). This multiplicity value is also obtained when using the more realistic reflection by a plasma mirror (reflected field shown in Fig. 3 of the Manuscript).

Such a good agreement between model and simulation comforts our claim that significant pair production can be achieved in this single-laser setup. It also shows that, for the parameters discussed here, the first generation of

---

[1] This result can be easily obtained using the tool made available online by the authors of Ref. [11]: `https://github.com/Syttam/Shower-multiplicity`.

produced pairs (the only one accounted for in the model of Ref. [11]) dominates the development of the shower.

---

[1] R. Lehe, M. Kirchen, I. A. Andriyash, B. B. Godfrey, and J.-L. Vay, A spectral, quasi-cylindrical and dispersion-free particle-in-cell algorithm, Comp. Phys. Commun. **203**, 66–82 (2016).

[2] S. Diederichs, C. Benedetti, A. Huebl, R. Lehe, A. Myers, A. Sinn, J.-L. Vay, W. Zhang, and M. Thévenet, Hipace++: A portable, 3d quasi-static particle-in-cell code, Comp. Phys. Commun. **278**, 108421 (2022).

[3] E. Lefebvre, N. Cochet, S. Fritzler, V. Malka, M.-M. A. onard, J.-F. Chemin, S. Darbon, L. Disdier, J. Faure, A. Fedotoff, O. Landoas, G. Malka, V. M. ot, P. Morel, M. R. L. Gloahec, A. Rouyer, C. Rubbelynck, V. Tikhonchuk, R. Wrobel, P. Audebert, and C. Rousseaux, Electron and photon production from relativistic laser–plasma interactions, Nucl. Fusion **43**, 629 (2003).

[4] M. Lobet, E. d'Humières, M. Grech, C. Ruyer, X. Davoine, and L. Gremillet, Modeling of radiative and quantum electrodynamics effects in PIC simulations of ultra-relativistic laser-plasma interaction, J. Phys.: Conf. Ser. **688**, 012058 (2016).

[5] S. Montefiori and M. Tamburini, Sfqedtoolkit: A high-performance library for the accurate modeling of strong-field qed processes in pic and monte carlo codes, Comp. Phys. Commun. **292**, 108855 (2023).

[6] E. Guillaume, *Control of electron injection and acceleration in Laser-Wakefield Accelerators*, Ph.D. thesis (2015), thèse de doctorat dirigée par Malka, Victor Physique Palaiseau, Ecole polytechnique 2015.

[7] M. Thévenet, I. Andriyash, L. Fedeli, A. Ferran Pousa, A. Huebl, S. Jalas, R. Lehe, and R. Shalloo, Lasy-org/lasy: 0.4.0 (2023).

[8] C. Benedetti, C. B. Schroeder, C. G. R. Geddes, E. Esarey, and W. P. Leemans, An accurate and efficient laser-envelope solver for the modeling of laser-plasma accelerators, Plasma Physics and Controlled Fusion **60**, 014002 (2017).

[9] T. C. DuBois, E. Siminos, J. Ferri, L. Gremillet, and T. Fülöp, Origins of plateau formation in ion energy spectra under target normal sheath acceleration, Physics of Plasmas **24**, 10.1063/1.5008806 (2017).

[10] R. Nuter *et al.*, Field ionization model implemented in particle in cell code and applied to laser-accelerated carbon ions, Physics of Plasmas **18**, 033107 (2011).

[11] M. Pouyez, A. A. Mironov, T. Grismayer, A. Mercuri-Baron, F. Perez, M. Vranic, C. Riconda, and M. Grech, Multiplicity of electron- and photon-seeded electromagnetic showers at multi-petawatt laser facilities, arXiv:2402.04501.
